# Supplementary material for: Dream-to-Recon: Monocular 3D Reconstruction with Diffusion-Depth Distillation from Single Images
Source: arXiv:2508.02323 source file (2025-08-04)
Supplement: Supplementary file 2 [file table_real_views.tex]

\begin{table*}[t]
    \centering
    % \footnotesize
    % UniDepth & 89\textsubscript{\textit{0.84}} & -- & -- & 96\textsubscript{\textit{0.34}} & -- & -- \\
    % Metric3D & 91\textsubscript{\textit{0.64}} & -- & -- & 97\textsubscript{\textit{0.24}} & -- & -- \\
    % \textbf{Ours} (minor bug) & {93}\textsubscript{\textit{0.49}} & {72}\textsubscript{\textit{3.51}} & {74}\textsubscript{\textit{6.67}} & {97}\textsubscript{\textit{0.35}} & {73}\textsubscript{\textit{6.82}} & {96}\textsubscript{\textit{1.35}} \\
\setlength{\tabcolsep}{4pt} % Slightly reduced from the default of 6pt
\begin{tabular}{clccc|ccc}
    \toprule
    & \textit{Method} & $\text{O}_\text{acc}$~$\uparrow$ & $\text{IE}_\text{acc}$~$\uparrow$ & $\text{IE}_\text{rec}$~$\uparrow$ & $\text{O}_\text{acc}$~$\uparrow$ & $\text{IE}_\text{acc}$~$\uparrow$ & $\text{IE}_\text{rec}$~$\uparrow$ \\
    \midrule
    \multirow{4}{*}{\textit{a)}} 
    & BTS & 92\textsubscript{\textit{0.64}} & 69\textsubscript{\textit{4.24}} & 64\textsubscript{\textit{8.37}} & 95\textsubscript{\textit{0.74}} & 63\textsubscript{\textit{10.71}} & 94\textsubscript{\textit{1.88}} \\
    & BTS-D & 92\textsubscript{\textit{0.70}} & 70\textsubscript{\textit{3.96}} & 66\textsubscript{\textit{8.24}} & 95\textsubscript{\textit{0.77}} & 61\textsubscript{\textit{11.66}} & 96\textsubscript{\textit{1.11}} \\
    \cmidrule(lr){2-8}
    & \textbf{Ours} & 93\textsubscript{\textit{0.49}} & 72\textsubscript{\textit{3.51}} & 74\textsubscript{\textit{6.67}} 
        & 97\textsubscript{\textit{0.35}} 
        & 73\textsubscript{\textit{6.82}} 
        & 96\textsubscript{\textit{1.35}} \\
    & \textbf{Ours} (Distilled) & 90\textsubscript{\textit{0.86}} & 71\textsubscript{\textit{3.84}} & 71\textsubscript{\textit{9.00}} & 96\textsubscript{\textit{0.43}} & 72\textsubscript{\textit{7.10}} & 93\textsubscript{\textit{2.69}} \\
    \midrule
    \multirow{2}{*}{\textit{b)}} 
    & \textbf{Ours} & 93\textsubscript{\textit{0.49}} & 72\textsubscript{\textit{3.51}} & 74\textsubscript{\textit{6.67}} 
        & 97\textsubscript{\textit{0.35}} 
        & 73\textsubscript{\textit{6.82}} 
        & 96\textsubscript{\textit{1.35}} \\
    & Ours w/ real MV & 93\textsubscript{\textit{0.50}} & 71\textsubscript{\textit{3.91}} & 66\textsubscript{\textit{7.62}} & 97\textsubscript{\textit{0.25}} & 71\textsubscript{\textit{7.07}} & 91\textsubscript{\textit{3.25}} \\
    \bottomrule
\end{tabular}
    \caption{\textbf{Scene Reconstruction.} \textit{a)} Results on KITTI-360 / Waymo in \% with variances. \textit{b)} Comparing synthesized views vs. real multi-view data for building the \pvol.
    }
    \label{tab:reb_reconstruction_quantitative}
\end{table*}
